# Supplementary material for: Avoid Catastrophic Forgetting with Rank-1 Fisher from Diffusion Models
Source: arXiv:2509.23593 source file (2026-01-26)
Supplement: Supplementary file 4 [file rank-1-analysis_small.tex]

% in your document where you want the three figures to appear
{\captionsetup[subfigure]{labelformat=parens,labelsep=space} % or labelformat=simple
% Requires: \usepackage{subcaption}
\begin{figure}[h!] % keep the quartet together
  \centering

  % \begin{subfigure}[t]{0.26\textwidth}
  %   \vspace{0pt}\centering
  %   \includegraphics[width=\linewidth]{plots/analysis/small-model/cosine_similarity_mu.pdf}
  %   \caption{}
  %   \label{fig:cos-mu}
  % \end{subfigure}\hfill
  \begin{subfigure}[t]{0.3\textwidth}
    \vspace{0pt}\centering
    \includegraphics[width=\linewidth]{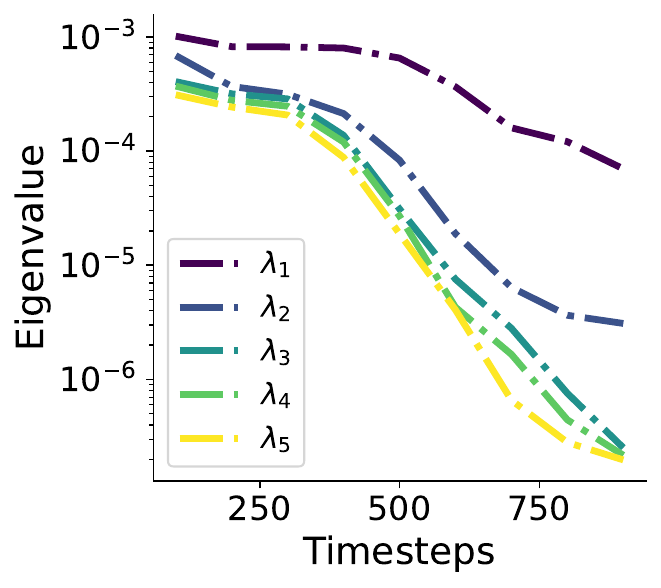}
    \caption{}
    \label{fig:top-eigs-small}
  \end{subfigure}\hfill
  \begin{subfigure}[t]{0.24\textwidth}
    \vspace{0pt}\centering
    \includegraphics[width=\linewidth]{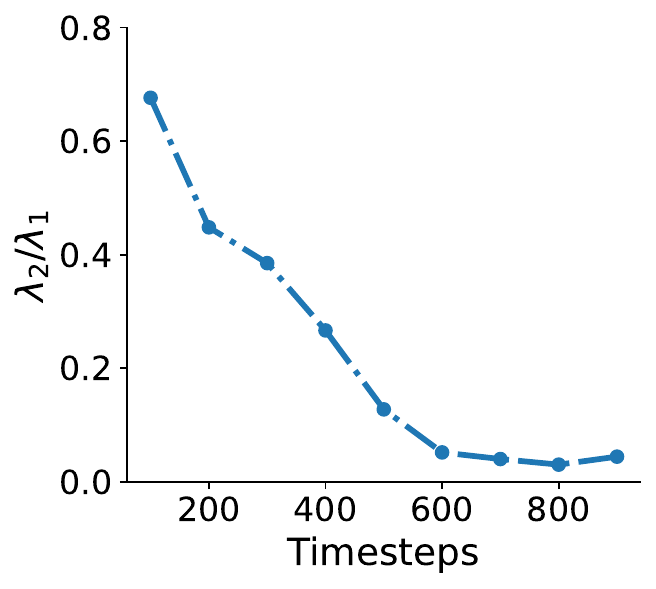}
    \caption{}
    \label{fig:eig-ratio-small}
  \end{subfigure}
  % \hfill
  % \begin{subfigure}[t]{0.24\textwidth}
  %   \vspace{0pt}\centering
  %   \includegraphics[width=\linewidth]{plots/analysis/small-model/frobenius.pdf}
  %   \caption{}
  %   \label{fig:f-norms}
  % \end{subfigure}
  \vspace{-10px}
  \caption{(a): Top 5 eigenvalues of $F_t(\theta)$ across timesteps in log-scale. (b): The ratio $r_t=\lambda_2/\lambda_1$ across timesteps. Small-1 Model}

\end{figure}

% \begin{figure}[b] % optional float so the trio stays together
%   \centering
%   \begin{minipage}[t]{0.24\textwidth}
%     \vspace{0pt}\centering
%     \includegraphics[width=1.028\linewidth]{plots/analysis/small-model/cosine_similarity_mu.pdf}
%     \captionof{figure}{Co.}
%     \label{fig:top-eig}
%   \end{minipage}\hfill
%   \begin{minipage}[t]{0.24\textwidth}
%     \vspace{0pt}\centering
%     \includegraphics[width=0.95\linewidth]{plots/analysis/small-model/top10_eigenvalues.pdf}
%     \captionof{figure}{Top 5 eigenvalues of $F(\theta)$ across timesteps (log-scale).}
%     \label{fig:top-eig}
%   \end{minipage}\hfill
%   \begin{minipage}[t]{0.24\textwidth}
%     \vspace{0pt}\centering
%     \includegraphics[width=0.95\linewidth]{plots/analysis/small-model/eigenvalue_ratio.pdf}
%     \captionof{figure}{Ratio $r_t=\lambda_2/\lambda_1$ across timesteps.}
%     \label{fig:eig-ratio}
%   \end{minipage}\hfill
%   \begin{minipage}[t]{0.24\textwidth}
%     \vspace{0pt}\centering
%     \includegraphics[width=0.95\linewidth]{plots/analysis/small-model/frobenius.pdf}
%     \captionof{figure}{Relative Frobenius norm between $F(\theta)$ and diagonal and rank-1 approximations.}
%     \label{fig:f-nroms}
%   \end{minipage}

% \end{figure}
